# Supplementary material for: Streaming Algorithms with Large Approximation Factors
Source: arXiv:2207.08075 source file (2022-07-17)
Supplement: Supplementary file 1 [file fp_reduction_appendix.tex]

\section{$\ell_p$ Estimation $p > 2$: A Reduction to Streaming} % :
\label{sec:ellp_reduction}
To lower bound the space complexity of a streaming algorithm we need a way of
relating it to the communication cost of a protocol for this communication problem. In~\cite{WW15}, the authors use a result of~\cite{lnw14}, which shows under certain conditions, any streaming algorithm $\mathcal{A}$ that solves the problem $P$ on any stream with probability at least $1 - \delta$ can be converted to a path-independent randomized automaton $\mathcal{B}$ that solves $P$ on $Z_{|m|}^n$ with probability at least $1-7\delta$, and the space complexity of $\mathcal{B}$ is the same as that of $\mathcal{A}$ up to a factor of $(\log n + \log\log m + \log 1/\delta)$. Here  path-independence means that the output of the algorithm only depends on the initial state and underlying frequency vector. In other words, the order of the updates of the same frequency vector will not cause different outputs of such an algorithm. We now assume that the algorithm $\mathcal{A}$ we have enjoys this path-independence property. From a more detailed discussion, we refer the readers to Section~5 in~\cite{WW15}.
\begin{theorem}[\cite{lnw14}, corollary of Theorem~10]\label{thm:path-independent}
Suppose that there is a streaming algorithm $\mathcal{A}$ that solves problem $P$ on any stream with probability at least $1 - \delta$. Then there is a path-independent randomized algorithm $\mathcal{B}$ that solve $P$ on $Z_{|m|}^n$ with probability at least $1-7\delta$, and the space complexity of $\mathcal{B}$ is $S(\mathcal{B}, m) \le S(\mathcal{A}, m) + O(\log n + \log\log m + \log 1/\delta)$.
\end{theorem}
Combining Theorem~\ref{thm:ww15} and Theorem~\ref{thm:path-independent}, we have
\begin{lemma}[\cite{WW15}, Corollary 5.7]
\label{lem:smp}
Let $P(x_1, ..., x_s)$ be an $s$-ary relation such that the symmetric SMP communication complexity of $P$ is $c$. Let $\mathcal{A}$ be a space-optimal streaming algorithm from which the output of $\mathcal{A}$ on an input stream $\sigma$ with the underlying vector $x$ can be used to solve $P$ with probability at least $1 - \delta$. Then the space complexity of $\mathcal{A}$ is at least $c/s$.
\end{lemma}
